# Supplementary material for: Depth Pro: Sharp Monocular Metric Depth in Less Than a Second
Source: arXiv:2410.02073 source file (2025-04-21)
Supplement: Supplementary file 1 [file sota.tex]

\begin{figure}[htbp]
  \centering
 	\begin{tabular}{cccc}
        Input & Depth Pro & Marigold & Metric3Dv2 \\
        \includegraphics[width=0.22\textwidth]{fig/quali/-TrR0EHsNzg.jpg} &
        \includegraphics[width=0.22\textwidth]{fig/quali/-TrR0EHsNzg.jpg_depthpro.png} &
        \includegraphics[width=0.22\textwidth]{fig/quali/-TrR0EHsNzg.jpg_marigold.png} &
        \includegraphics[width=0.22\textwidth]{fig/quali/-TrR0EHsNzg.jpg_metric3d.png} \\
        \includegraphics[width=0.22\textwidth]{fig/quali/0XUvCVtnxYk.jpg} &
        \includegraphics[width=0.22\textwidth]{fig/quali/0XUvCVtnxYk.jpg_depthpro.png} &
        \includegraphics[width=0.22\textwidth]{fig/quali/0XUvCVtnxYk.jpg_marigold.png} &
        \includegraphics[width=0.22\textwidth]{fig/quali/0XUvCVtnxYk.jpg_metric3d.png} \\
        \includegraphics[width=0.22\textwidth]{fig/quali/0QFUAbRlGFY.jpg} &
        \includegraphics[width=0.22\textwidth]{fig/quali/0QFUAbRlGFY.jpg_depthpro.png} &
        \includegraphics[width=0.22\textwidth]{fig/quali/0QFUAbRlGFY.jpg_marigold.png} &
        \includegraphics[width=0.22\textwidth]{fig/quali/0QFUAbRlGFY.jpg_metric3d.png} \\
        \includegraphics[width=0.22\textwidth]{fig/quali/0-IKoef3Ukw.jpg} &
        \includegraphics[width=0.22\textwidth]{fig/quali/0-IKoef3Ukw_depthpro.png} &
        \includegraphics[width=0.22\textwidth]{fig/quali/0-IKoef3Ukw_marigold.png} &
        \includegraphics[width=0.22\textwidth]{fig/quali/0-IKoef3Ukw_metric3d.png} \\
        \includegraphics[width=0.22\textwidth]{fig/quali/1Z6kBIa7QPc.jpg} &
        \includegraphics[width=0.22\textwidth]{fig/quali/1Z6kBIa7QPc.jpg_depthpro.png} &
        \includegraphics[width=0.22\textwidth]{fig/quali/1Z6kBIa7QPc.jpg_marigold.png} &
        \includegraphics[width=0.22\textwidth]{fig/quali/1Z6kBIa7QPc.jpg_metric3d.png} \\
        \includegraphics[width=0.22\textwidth]{fig/quali/-TLWOLpkd3o.jpg} &
        \includegraphics[width=0.22\textwidth]{fig/quali/-TLWOLpkd3o.jpg_depthpro.png} &
        \includegraphics[width=0.22\textwidth]{fig/quali/-TLWOLpkd3o.jpg_marigold.png} &
        \includegraphics[width=0.22\textwidth]{fig/quali/-TLWOLpkd3o.jpg_metric3d.png} \\
        \includegraphics[width=0.22\textwidth]{fig/quali/_-V3wzssibE.jpg} &
        \includegraphics[width=0.22\textwidth]{fig/quali/_-V3wzssibE.jpg_depthpro.png} &
        \includegraphics[width=0.22\textwidth]{fig/quali/_-V3wzssibE.jpg_marigold.png} &
        \includegraphics[width=0.22\textwidth]{fig/quali/_-V3wzssibE.jpg_metric3d.png} \\
        \includegraphics[width=0.22\textwidth]{fig/quali/2d07bhKmsvs.jpg} &
        \includegraphics[width=0.22\textwidth]{fig/quali/2d07bhKmsvs.jpg_depthpro.png} &
        \includegraphics[width=0.22\textwidth]{fig/quali/2d07bhKmsvs.jpg_marigold.png} &
        \includegraphics[width=0.22\textwidth]{fig/quali/2d07bhKmsvs.jpg_metric3d.png} \\
        \includegraphics[width=0.22\textwidth]{fig/quali/-W3oWqvkfg8.jpg} &
        \includegraphics[width=0.22\textwidth]{fig/quali/-W3oWqvkfg8.jpg_depthpro.png} &
        \includegraphics[width=0.22\textwidth]{fig/quali/-W3oWqvkfg8.jpg_marigold.png} &
        \includegraphics[width=0.22\textwidth]{fig/quali/-W3oWqvkfg8.jpg_metric3d.png} \\
    \end{tabular}
  \caption{.}
  \label{fig:supp_sota}
\end{figure}
  \vspace{7mm}

\begin{figure}[htbp]
  \centering
 	\begin{tabular}{cccc}
        Input & Depth Pro & Marigold & Metric3Dv2 \\
        \includegraphics[width=0.22\textwidth]{fig/quali/1DNsw53dqJw.jpg} &
        \includegraphics[width=0.22\textwidth]{fig/quali/1DNsw53dqJw.jpg_depthpro.png} &
        \includegraphics[width=0.22\textwidth]{fig/quali/1DNsw53dqJw.jpg_marigold.png} &
        \includegraphics[width=0.22\textwidth]{fig/quali/1DNsw53dqJw.jpg_metric3d.png} \\
        \includegraphics[width=0.22\textwidth]{fig/quali/-uZ08UybO7M.jpg} &
        \includegraphics[width=0.22\textwidth]{fig/quali/-uZ08UybO7M.jpg_depthpro.png} &
        \includegraphics[width=0.22\textwidth]{fig/quali/-uZ08UybO7M.jpg_marigold.png} &
        \includegraphics[width=0.22\textwidth]{fig/quali/-uZ08UybO7M.jpg_metric3d.png} \\
        \includegraphics[width=0.22\textwidth]{fig/quali/-dKnvCH-nBY.jpg} &
        \includegraphics[width=0.22\textwidth]{fig/quali/-dKnvCH-nBY_depthpro.png} &
        \includegraphics[width=0.22\textwidth]{fig/quali/-dKnvCH-nBY_marigold.png} &
        \includegraphics[width=0.22\textwidth]{fig/quali/-dKnvCH-nBY_metric3d.png} \\
        \includegraphics[width=0.22\textwidth]{fig/quali/-ZzUG65jTKU.jpg} &
        \includegraphics[width=0.22\textwidth]{fig/quali/-ZzUG65jTKU.jpg_depthpro.png} &
        \includegraphics[width=0.22\textwidth]{fig/quali/-ZzUG65jTKU.jpg_marigold.png} &
        \includegraphics[width=0.22\textwidth]{fig/quali/-ZzUG65jTKU.jpg_metric3d.png} \\
        \includegraphics[width=0.22\textwidth]{fig/quali/_-AgFr7hXds.jpg} &
        \includegraphics[width=0.22\textwidth]{fig/quali/_-AgFr7hXds.jpg_depthpro.png} &
        \includegraphics[width=0.22\textwidth]{fig/quali/_-AgFr7hXds.jpg_marigold.png} &
        \includegraphics[width=0.22\textwidth]{fig/quali/_-AgFr7hXds.jpg_metric3d.png} \\
        \includegraphics[width=0.22\textwidth]{fig/quali/0U2_xhUaLtQ.jpg} &
        \includegraphics[width=0.22\textwidth]{fig/quali/0U2_xhUaLtQ.jpg_depthpro.png} &
        \includegraphics[width=0.22\textwidth]{fig/quali/0U2_xhUaLtQ.jpg_marigold.png} &
        \includegraphics[width=0.22\textwidth]{fig/quali/0U2_xhUaLtQ.jpg_metric3d.png} \\
        \includegraphics[width=0.22\textwidth]{fig/quali/0uN9iF4mgDI.jpg} &
        \includegraphics[width=0.22\textwidth]{fig/quali/0uN9iF4mgDI.jpg_depthpro.png} &
        \includegraphics[width=0.22\textwidth]{fig/quali/0uN9iF4mgDI.jpg_marigold.png} &
        \includegraphics[width=0.22\textwidth]{fig/quali/0uN9iF4mgDI.jpg_metric3d.png} \\
        \includegraphics[width=0.22\textwidth]{fig/quali/-GfXCKvu7PA.jpg} &
        \includegraphics[width=0.22\textwidth]{fig/quali/-GfXCKvu7PA.jpg_depthpro.png} &
        \includegraphics[width=0.22\textwidth]{fig/quali/-GfXCKvu7PA.jpg_marigold.png} &
        \includegraphics[width=0.22\textwidth]{fig/quali/-GfXCKvu7PA.jpg_metric3d.png} \\
    \end{tabular}
  \caption{.}
  \label{fig:supp_sota1}
\end{figure}
  \vspace{7mm}

\begin{figure}[htbp]
  \centering
 	\begin{tabular}{cccc}
        Input & Depth Pro & Marigold & Metric3Dv2 \\
        \includegraphics[width=0.22\textwidth]{fig/quali/-5TVdPGk89E.jpg} &
        \includegraphics[width=0.22\textwidth]{fig/quali/-5TVdPGk89E.jpg_depthpro.png} &
        \includegraphics[width=0.22\textwidth]{fig/quali/-5TVdPGk89E.jpg_marigold.png} &
        \includegraphics[width=0.22\textwidth]{fig/quali/-5TVdPGk89E.jpg_metric3d.png} \\
        \includegraphics[width=0.22\textwidth]{fig/quali/-7JlKYhsVRU.jpg} &
        \includegraphics[width=0.22\textwidth]{fig/quali/-7JlKYhsVRU.jpg_depthpro.png} &
        \includegraphics[width=0.22\textwidth]{fig/quali/-7JlKYhsVRU.jpg_marigold.png} &
        \includegraphics[width=0.22\textwidth]{fig/quali/-7JlKYhsVRU.jpg_metric3d.png} \\
        \includegraphics[width=0.22\textwidth]{fig/quali/0DzBj1uz0wc.jpg} &
        \includegraphics[width=0.22\textwidth]{fig/quali/0DzBj1uz0wc_depthpro.png} &
        \includegraphics[width=0.22\textwidth]{fig/quali/0DzBj1uz0wc_marigold.png} &
        \includegraphics[width=0.22\textwidth]{fig/quali/0DzBj1uz0wc_metric3d.png} \\
        \includegraphics[width=0.22\textwidth]{fig/quali/_-9uiWbeftw.jpg} &
        \includegraphics[width=0.22\textwidth]{fig/quali/_-9uiWbeftw.jpg_depthpro.png} &
        \includegraphics[width=0.22\textwidth]{fig/quali/_-9uiWbeftw.jpg_marigold.png} &
        \includegraphics[width=0.22\textwidth]{fig/quali/_-9uiWbeftw.jpg_metric3d.png} \\
        \includegraphics[width=0.22\textwidth]{fig/quali/_2-L01zd-gc.jpg} &
        \includegraphics[width=0.22\textwidth]{fig/quali/_2-L01zd-gc.jpg_depthpro.png} &
        \includegraphics[width=0.22\textwidth]{fig/quali/_2-L01zd-gc.jpg_marigold.png} &
        \includegraphics[width=0.22\textwidth]{fig/quali/_2-L01zd-gc.jpg_metric3d.png} \\
        \includegraphics[width=0.22\textwidth]{fig/quali/_24x_8lBIOk.jpg} &
        \includegraphics[width=0.22\textwidth]{fig/quali/_24x_8lBIOk.jpg_depthpro.png} &
        \includegraphics[width=0.22\textwidth]{fig/quali/_24x_8lBIOk.jpg_marigold.png} &
        \includegraphics[width=0.22\textwidth]{fig/quali/_24x_8lBIOk.jpg_metric3d.png} \\
        \includegraphics[width=0.22\textwidth]{fig/quali/_11vc8DgTGU.jpg} &
        \includegraphics[width=0.22\textwidth]{fig/quali/_11vc8DgTGU.jpg_depthpro.png} &
        \includegraphics[width=0.22\textwidth]{fig/quali/_11vc8DgTGU.jpg_marigold.png} &
        \includegraphics[width=0.22\textwidth]{fig/quali/_11vc8DgTGU.jpg_metric3d.png} \\
        \includegraphics[width=0.22\textwidth]{fig/quali/_07o67_KJ_Y.jpg} &
        \includegraphics[width=0.22\textwidth]{fig/quali/_07o67_KJ_Y.jpg_depthpro.png} &
        \includegraphics[width=0.22\textwidth]{fig/quali/_07o67_KJ_Y.jpg_marigold.png} &
        \includegraphics[width=0.22\textwidth]{fig/quali/_07o67_KJ_Y.jpg_metric3d.png} \\
    \end{tabular}
  \caption{.}
  \label{fig:supp_sota2}
\end{figure}
  \vspace{7mm}
