# Supplementary material for: Depth Pro: Sharp Monocular Metric Depth in Less Than a Second
Source: arXiv:2410.02073 source file (2025-04-21)
Supplement: Supplementary file 2 [file best_backbones384.tex]

\begin{table}[htbp]
  \label{tab:best_backbones384}
  \centering
  \begin{tabular}{@{}lllllll@{}}
    \toprule
    Backbone & AbsRel $\downarrow$ & Log10 $\downarrow$ & Edge-0 $\downarrow$ & Edge-1 $\downarrow$ & Avg-rank $\downarrow$\\
    \midrule
    beitv2l16~\cite{Peng2022:arxiv} & 5 & 3 & \bf{1} & 3 & \bf{3.0}\\
    vitl16-mae~\cite{He2022:CVPR} & 4 & 6 & 3 & \bf{1} & \underline{3.5}\\
    dinov2l16~\cite{Oquab2024:arxiv} & 3 & \underline{2} & 9 & 6 & 5.0\\
    dinov2l16-reg4~\cite{Oquab2024:arxiv} & \underline{2} & 4 & 8 & 8 & 5.5\\
    clip-quickgelu~\cite{Radford2021:arxiv} & 8 & 9 & \underline{2} & \underline{2} & 5.5\\
    eva0216-clip~\cite{Sun2023:arxiv} & \bf{1} & \bf{1} & 13 & 10 & 6.25\\
    vitl16~\cite{Dosovitskiy2021:ICLR}  & 10 & 9 & 10 & 4 & 8.3\\  
  \bottomrule
  \end{tabular}
  \caption{Ranks of 7 the best backbones with 384$\times$384 resolution trained on 5 RGB-D datasets: Keystone, HRWSI, RedWeb, TartanAir, Hypersim.
  }
\end{table}
