# Supplementary material for: Depth Pro: Sharp Monocular Metric Depth in Less Than a Second
Source: arXiv:2410.02073 source file (2025-04-21)
Supplement: Supplementary file 3 [file trainingsets.tex]

\begin{table}[htbp]
  \label{tab:datasets}
  \centering
  \begin{tabular}{@{}lllllll@{}}
    \toprule
    Backbone & \multicolumn{1}{p{1.7cm}}{labels} & distillation & Samples & Datasets\\
    \midrule
    beitv2l16~\cite{Peng2022:arxiv} & $\checkmark$ & $\checkmark$ & 400 M & ImageNet1k, CLIP for VQ-KD\\
    vitl16-mae~\cite{He2022:CVPR} & - & - & 1.4 M & ImageNet1k\\
    dinov2l16~\cite{Oquab2024:arxiv} & - & $\checkmark$ & 142 M & LVD-142M curated dataset\\
    dinov2l16-reg4~\cite{Oquab2024:arxiv} & - & $\checkmark$ & 142 M & LVD-142M curated dataset\\
    clip-quickgelu~\cite{Radford2021:arxiv} & $\checkmark$ & - & 400 M & CLIP\\
    eva0216-clip~\cite{Sun2023:arxiv} & $\checkmark$ & $\checkmark$ & $\sim$ 3 B  & \multicolumn{1}{p{4.0cm}}{LAION-2B, COYO-700M, IN-21K, CC12M, CC3M, COCO, ADE20K, Object365, OpenImages}\\
    vitl16~\cite{Dosovitskiy2021:ICLR} & $\checkmark$ & - & 14 M  & ImageNet21k\\
  \bottomrule
  \end{tabular}
  \caption{Training datasets for 7 the best backbones.
  }
\end{table}
